# Supplementary material for: Exchange-enhanced Ultrastrong Magnon-Magnon Coupling in a Compensated Ferrimagnet
Source: arXiv:1903.04330 ancillary file (2019-09-23)
Supplement: Supplementary file 1 [file GdIG_Tunable_Coupling_SI.pdf]

# Supplemental Material: Exchange-enhanced Ultrastrong Magnon-Magnon Coupling in a Compensated Ferrimagnet

Lukas Liensberger,<sup>1,2,\*</sup> Akashdeep Kamra,<sup>3,†</sup> Hannes Maier-Flaig,<sup>1,2</sup> Stephan Geprägs,<sup>1</sup> Andreas Erb,<sup>1</sup> Sebastian T. B. Goennenwein,<sup>4</sup> Rudolf Gross,<sup>1,2,5,6</sup> Wolfgang Belzig,<sup>7</sup> Hans Huebl,<sup>1,2,5,6</sup> and Mathias Weiler<sup>1,2,‡</sup>

<sup>1</sup>*Walther-Meißner-Institut, Bayerische Akademie der Wissenschaften, 85748 Garching, Germany*

<sup>2</sup>*Physik-Department, Technische Universität München, 85748 Garching, Germany*

<sup>3</sup>*Center for Quantum Spintronics, Department of Physics,*

*Norwegian University of Science and Technology, 7491 Trondheim, Norway*

<sup>4</sup>*Institut für Festkörper- und Materialphysik, Technische Universität Dresden, 01062 Dresden, Germany*

<sup>5</sup>*Nanosystems Initiative Munich, 80799 Munich, Germany*

<sup>6</sup>*Munich Center for Quantum Science and Technology (MCQST), 80799 Munich, Germany*

<sup>7</sup>*Department of Physics, University of Konstanz, 78457 Konstanz, Germany*

(Dated: August 16, 2019)

## MATERIAL

Gadolinium iron garnet ( $\text{Gd}_3\text{Fe}_5\text{O}_{12}$ , GdIG) is a compensated ferrimagnet consisting of three magnetic sublattices. The two nearly temperature-independent iron-sublattice magnetizations couple strongly antiferromagnetically to each other. They can be treated as one effective iron-sublattice. GdIG features a strongly temperature-dependent gadolinium-sublattice magnetization which is antiferromagnetically coupled to the iron-sublattice [1] in the considered temperature and magnetic field range, resulting in an effective two-sublattice system. Due to the temperature-dependence of the Gd-sublattice a compensation of the sublattice magnetizations occurs, where the net remanent magnetization vanishes at the so-called magnetic compensation temperature  $T_{\text{comp}}$  which we determined by SQUID magnetometry measurements to  $T_{\text{comp}} = 288$  K.

The single crystal GdIG disk was grown using traveling solvent floating zone method [2] and cut to a (111)-oriented disk with diameter  $d = 6.35$  mm and thickness  $t = 500$   $\mu\text{m}$ .

## SUBLATTICE MAGNETIZATIONS AND SQUID MAGNETOMETRY MEASUREMENTS

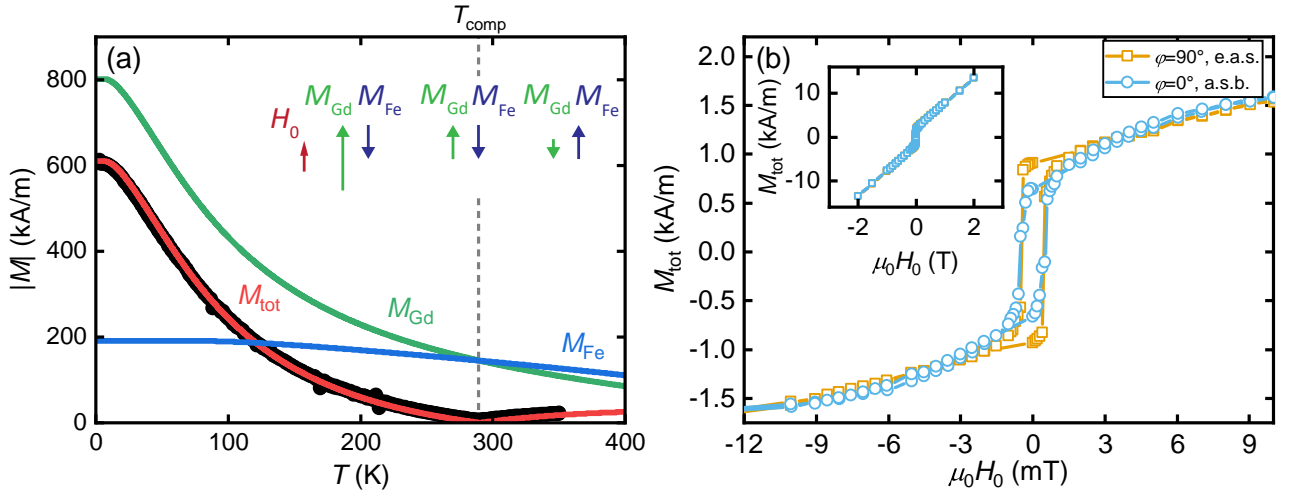

FIG. S1. (a) Simulated static magnetizations of gadolinium (green solid line) and iron (blue solid line) sublattices vs. temperature. The measured total magnetization  $M_{\text{tot}}$  carried out in a magnetic field of  $\mu_0 H_0 = 1.0$  T is shown by black circles. The insets schematically depict the sublattice magnetizations. (b) Measured magnetic field-dependence of the total magnetization  $M_{\text{tot}}$  along the e.a.s. (orange) and a.s.b. (blue) direction at  $T = 282$  K. The inset shows the full SQUID magnetometry measurement up to 2 T.

The three sublattices of the rare-earth iron garnet GdIG add up to the total magnetization

$$M_{\text{tot}} = M_{\text{Gd}} + M_{\text{Fe,a}} - M_{\text{Fe,d}} = M_{\text{Gd}} + M_{\text{Fe}}. \quad (\text{S1})$$

The two iron sublattices (a- and d-site) are strongly antiferromagnetically coupled and can be treated as one effective iron sublattice  $M_{\text{Fe}} = M_{\text{Fe,a}} - M_{\text{Fe,d}}$ . Therefore, the effective number of sublattices is reduced from three to two. The gadolinium sublattice (c-site) is weakly antiferromagnetically coupled to the net iron sublattice, which leads to the emergence of the magnetic compensation point at  $T_{\text{comp}}$ , where the remanent magnetization of the Gd sublattice equals that of the net iron sublattice  $|M_{\text{Gd}}| = |M_{\text{Fe}}|$ .

The calculation of the sublattice magnetizations at non-zero temperatures can be done by using molecular field theory, where we follow the approach proposed in Refs. [3] and [4] in which all three sublattices are considered. The magnetization  $M_i$  of the three sublattices is given by

$$M_i(T) = M_i(0) \cdot B_{S_i}(a_i), \quad i \in \{a, d, c\} \quad (\text{S2})$$

with  $a=\text{Fe}_a$ ,  $d=\text{Fe}_d$ , and  $c=\text{Gd}$ . Here,  $M_i(0)$  is the magnetization at  $T = 0$  K and  $B_{S_i}(a_i)$  is the Brillouin function

with the Boltzmann energy ratios

$$\begin{aligned} a_d &= \frac{S_d g \mu_B \mu_0}{k_B T} \cdot (N_{dd} M_d + N_{da} M_a + N_{dc} M_c), \\ a_a &= \frac{S_a g \mu_B \mu_0}{k_B T} \cdot (N_{ad} M_d + N_{aa} M_a + N_{ac} M_c), \\ a_c &= \frac{J_c g \mu_B \mu_0}{k_B T} \cdot (N_{cd} M_d + N_{ca} M_a + N_{cc} M_c), \end{aligned} \quad (S3)$$

where the coupling between the sublattices has been taken into account. Here,  $S_d = S_a = 5/2$  is the spin angular momentum of the iron-sublattices and  $J_c = 7/2$  is the angular momentum of the Gd-sublattice [1],  $k_B$  is the Boltzmann constant and  $g = 2$  is the Landé factor. The sublattice magnetizations  $M_i$  at  $T = 0$  are given by [4]

$$\begin{aligned} M_d(0) &= 3gS_d\mu_B N_A, \\ M_a(0) &= 2gS_a\mu_B N_A, \\ M_c(0) &= 3gJ_c\mu_B N_A, \end{aligned} \quad (S4)$$

where  $\mu_B$  is the Bohr magneton and  $N_A$  is the Avogadro constant. The molecular field coefficients  $N_i$  are taken from Ref. [4], where we slightly adjusted  $N_{ac}$  from  $-3.44 \text{ mol/cm}^3$  to  $-3.3 \text{ mol/cm}^3$ . All remaining  $N_i$  are identical to those in Ref. [4] to yield the compensation temperature  $T_{\text{comp}} = 288 \text{ K}$  found in the SQUID magnetometry measurements (see Fig. S1, black circles). By solving the set of equations (S3), the magnetization of the sublattices  $M_i$  and the total magnetization  $M_{\text{tot}}$  can be calculated, which are shown in Fig. S1 as solid lines. Below the compensation point  $T < T_{\text{comp}}$ , the magnetization of the gadolinium sublattice  $M_{\text{Gd}}$  is larger than that of the net iron sublattice  $M_{\text{Fe}}$ , while the magnetization of the net iron sublattice dominates at  $T > T_{\text{comp}}$  (see inset in Fig. S1). The calculated total magnetization  $M_{\text{tot}}$  is in good agreement with the measured SQUID data.

Additionally, we measured the magnetic field dependence of the total magnetization  $M_{\text{tot}}$  at  $T = 282 \text{ K}$  as shown in Fig. S1(b). We observe the expected hysteresis loop due to the switching of the total magnetization. Comparing the two directions in the (111)-plane of the GdIG-disk (e.a.s and a.s.b.), it can be seen from the shape of the hysteresis that along the e.a.s., the curve “jumps” at the coercive field as expected for an easy axis in a Stoner-Wolfarth model [5]. Along the a.s.b. direction, the hysteresis is more rounded at the coercive field which in comparison to the e.a.s. direction is a magnetic harder axis. This small difference stems from the small cubic anisotropy as discussed below.

## BROADBAND MAGNETIC RESONANCE MEASUREMENTS BELOW AND ABOVE THE COMPENSATION TEMPERATURE

In Fig. S2, broadband magnetic resonance measurements at three different temperatures (280 K, 282 K, 294 K) with the magnetic field along the effectively axially symmetric (e.a.s.) and axial symmetry broken (a.s.b.) direction respectively are shown. In our experiments we measure the transmission magnitude  $S_{21}$  through a coplanar waveguide on which the GdIG-disk is placed as a function of microwave frequency  $f$  and magnetic field  $H_0$ . We then calculate the background corrected magnetic field derivative [6]

$$\partial_D S_{21} / \partial H_0 = \frac{S_{21}(H_0 + \Delta H) - S_{21}(H_0 - \Delta H)}{S_{21}(H_0) \Delta H}, \quad (S5)$$

where  $\Delta H$  is the fixed magnetic field step, which in our case is  $10 \text{ mT}/\mu_0$ . First, comparing the measurement results below the compensation point ( $T < T_{\text{comp}}$ ). With the magnetic field applied along the effectively axial symmetric direction [Figs. S2 (a) and (c)], we observe a shift of the spin-down mode to higher resonance frequencies with decreasing temperature. In the axial symmetry broken case [Figs. S2 (b) and (d)] we observe the anti-crossing of the two resonance modes at both temperatures, although the coupling gets smaller for  $T = 280 \text{ K}$ . The main text presents the case of  $T = 282 \text{ K}$  where the ultrastrong coupling along the hard axis is more pronounced with a normalized coupling strength  $\eta(282 \text{ K}) = g_c/(2\pi f_c) = 0.37$  in contrast to  $\eta(280 \text{ K}) = 0.24$ . Comparing these results taken below the compensation point  $T_{\text{comp}}$  with the situation above the compensation temperature  $T = 294 \text{ K}$  ( $> T_{\text{comp}}$ ) [Figs. S2(e) and (f)], we see that the physics remain unchanged and we still observe the ultrastrong coupling along the a.s.b. direction. The dashed lines are the results of the numerical simulations with parameters given in Table S1. We denote the orange line as the high frequency and the black line as the low frequency branch.

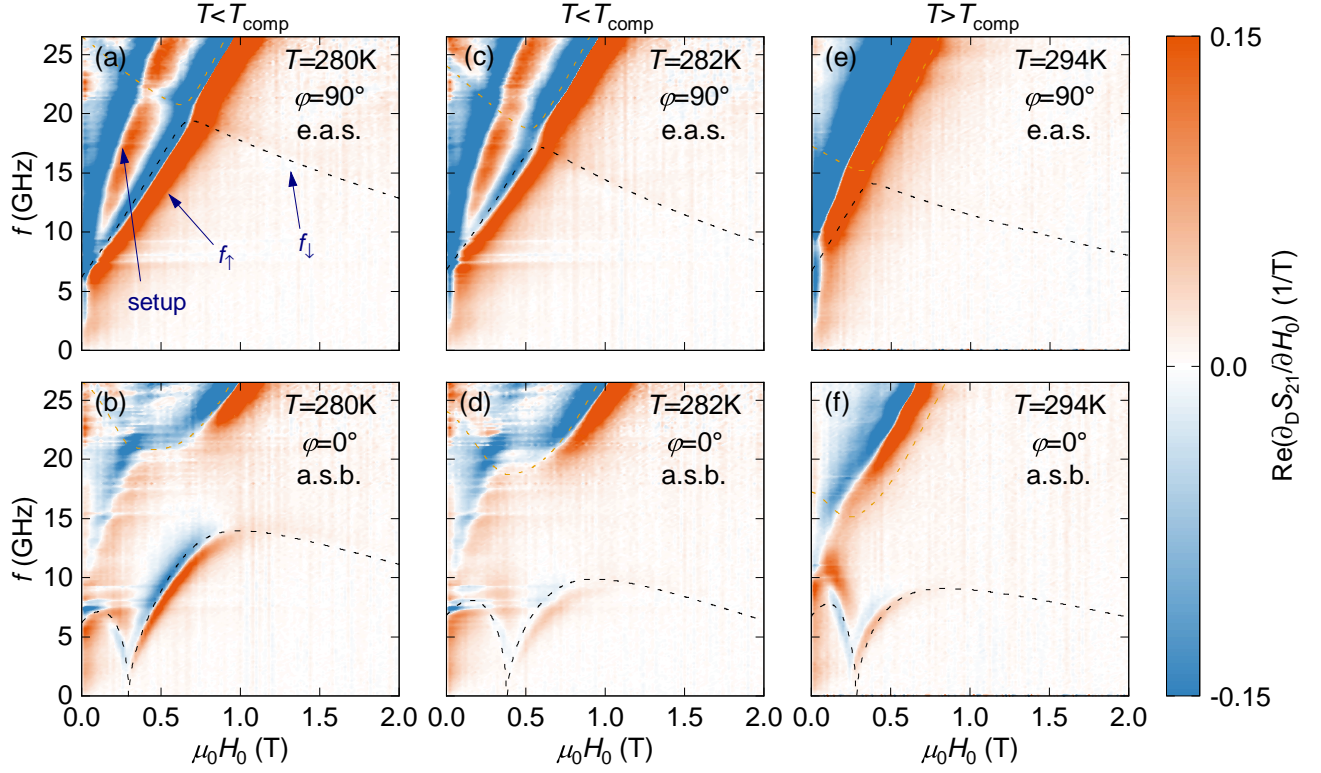

FIG. S2. Real part of the normalized magnetic field derivative of the complex transmission magnitude  $\text{Re } \partial_{\text{D}} S_{21} / \partial H_0$ , in a broadband ferromagnetic resonance measurement as a function of the static external magnetic field and the microwave frequency at (a),(b)  $T = 280$  K, (c),(d)  $T = 282$  K and (e),(f)  $T = 294$  K. The external magnetic field is applied (a),(c),(e) along the effectively axial symmetric (e.a.s.) direction  $\varphi = 90^\circ$ , where weak coupling between the two resonance modes is observed, and (b),(d),(f) along the axial symmetry broken (a.s.b.) axis  $\varphi = 0^\circ$  where the resonances interact ultrastrongly and exhibit an anti-crossing behavior. In all cases, the resonance seen at low fields stems from a magnetic compound in the setup and not from the sample. The dashed black and orange lines are the results from the numerical simulations.

For the rotations at fixed magnitude  $H_0$  in Figs. 3(a) and (b) in the main text, we use

$$\partial_{\text{D}} S_{21} / \partial \varphi = \frac{S_{21}(\omega, H_0, \varphi + \Delta\varphi) - S_{21}(\omega, H_0, \varphi - \Delta\varphi)}{S_{21}(\omega, H_0, \varphi) \cdot \Delta\varphi}, \quad (\text{S6})$$

where  $\Delta\varphi$  is the angle step size, which in our case is  $1^\circ$ .

### FITTING ROUTINE

In order to quantitatively extract the resonance frequencies  $\omega_i = 2\pi f_i$  and the half-width-at-half-maximum linewidths  $\kappa_i$ , the real and imaginary part of  $\partial_{\text{D}} S_{21} / \partial H_0$  are fitted at fixed magnetic field to [6, 7]

$$\partial_{\text{D}} S_{21} / \partial H_0|_{H_0} = \sum_{i=1}^2 \left[ A'_i \frac{\chi_i(\omega, H_0 + \Delta H) - \chi_i(\omega, H_0 - \Delta H)}{(A'_i \chi_i(\omega, H_0) + 1) \cdot \Delta H} \right] + C, \quad (\text{S7})$$

where  $A'_i$  are complex amplitudes,  $\chi_i$  are diagonal components of the Polder susceptibility, which describe the response of the dynamical component of the magnetization to an external oscillating magnetic field [8],  $\Delta H$  is the field step size of  $10 \text{ mT} / \mu_0$  and  $C = C_0 + C_1 H_0$  is a complex linear offset. For the fitting, we use for the susceptibility normalized to the saturation magnetization [6]

$$\chi_i(\omega, H_0) = \frac{|\gamma'| \mu_0 H_0 - i 2 \kappa_i}{\omega_i^2 - \omega^2 - i \omega 2 \kappa_i}. \quad (\text{S8})$$

with  $|\gamma'|$  the gyromagnetic ratio.

## NUMERICAL MODEL

Our numerical analysis follows the approach by Dreher *et al.* [9]. We start with the free energy density

$$F = J \mathbf{M}_A \cdot \mathbf{M}_B - \mu_0 \mathbf{H}_0 \cdot (\mathbf{M}_A + \mathbf{M}_B) + \frac{\mu_0}{2} (\mathbf{M}_A + \mathbf{M}_B) \overset{\leftrightarrow}{N} (\mathbf{M}_A + \mathbf{M}_B) + K_{c1} (\alpha_A^2 \beta_A^2 + \alpha_A^2 \delta_A^2 + \beta_A^2 \delta_A^2 + \alpha_B^2 \beta_B^2 + \alpha_B^2 \delta_B^2 + \beta_B^2 \delta_B^2) + K_{c2} (\alpha_A^2 \beta_A^2 \delta_A^2 + \alpha_B^2 \beta_B^2 \delta_B^2), \quad (\text{S9})$$

where  $\alpha_{A,B}$ ,  $\beta_{A,B}$  and  $\delta_{A,B}$  are the direction cosines of the magnetizations  $\mathbf{M}_{A,B}$  with respect to the cubic (100)-axes,  $J$  is the intersublattice antiferromagnetic exchange constant,  $\overset{\leftrightarrow}{N}$  is the demagnetization tensor for the disk-shaped sample [10], and  $K_{c1}$  and  $K_{c2}$  are the 1st and 2nd order cubic anisotropy constants. The subscripts A and B refer to the Gd- and Fe-sublattices, respectively. The lengths of the  $\mathbf{M}_{A,B}$  vectors are the saturation magnetizations  $M_B^s = M_{B0}$  and  $M_A^s = M_{A0} + \chi_a H_0$ , where we account for a field-dependent Gd-magnetization. For the plot of  $F$  in Fig. 3(c) in the main text, we set  $M_{B0} = 0$  and  $M_{A0} = 10 \text{ mT}/\mu_0$ .

To evaluate the magnetization dynamics, the free energy density is transformed to individual coordinate systems for the  $M_A$ - and  $M_B$ -sublattices, where the 3-axis is chosen along the equilibrium orientation of the respective sublattice magnetizations [9], while the 1- and 2-axes are along the dynamic components of  $\mathbf{M}_{A,B}$ . We use an harmonic Ansatz ( $M_{1,2} = m_{1,2} e^{i\omega t}$  and  $M_3 = M_{A,B}^s$ ) to solve the linearized coupled Landau-Lifshitz equations

$$\begin{aligned} \frac{\partial \mathbf{M}_A}{\partial t} &= -|\gamma_A| \mu_0 \mathbf{M}_A \times \mathbf{H}_{\text{eff},A}, \\ \frac{\partial \mathbf{M}_B}{\partial t} &= -|\gamma_B| \mu_0 \mathbf{M}_B \times \mathbf{H}_{\text{eff},B}, \end{aligned} \quad (\text{S10})$$

where  $\gamma_{A,B}$  are the gyromagnetic ratios, assumed negative, of the respective sublattice magnetizations. The effective magnetic fields  $\mathbf{H}_{\text{eff},A}$  and  $\mathbf{H}_{\text{eff},B}$  are given by

$$\begin{aligned} \mu_0 \mathbf{H}_{\text{eff},A} &= -\frac{\partial F}{\partial \mathbf{M}_A}, \\ \mu_0 \mathbf{H}_{\text{eff},B} &= -\frac{\partial F}{\partial \mathbf{M}_B}. \end{aligned} \quad (\text{S11})$$

We formulate the eigenvalue problem in the form  $\tilde{\chi}^{-1} \tilde{m}' = 0$ , where  $\tilde{m}'^\top = [m_{A,1} \ m_{A,2} \ m_{B,1} \ m_{B,2}]$  and the susceptibility  $\tilde{\chi}$  is a  $4 \times 4$  matrix. Resonance frequencies are obtained by setting  $\det \tilde{\chi}^{-1} = 0$  and solving for  $\omega$ . The parameters used for the simulation are summarized in the supplementary Table S1.

## FREE ENERGY CONTOURS AND PARAMETERS FOR THE NUMERICAL MODEL

The free energy density  $F$ , given by Eq. (S9), is plotted in Fig. S3(a) using the parameters compiled in Tab. S1, where the  $z$ -axis corresponds to the [111]-direction. In the top-down view shown in Fig. S3(b) it becomes evident that the [111]-direction is a crystalline easy axis and that the crystalline hard axes in the upper and lower plane are shifted by  $60^\circ$  with respect to each other. For the geometry relevant to our experiments, where the [111]-direction is pointing perpendicular to the disk plane, we consider the change of the free energy  $F$  in the disk plane as a function of the in-plane angle  $\varphi$  as shown in Fig. S3(e). For  $K_{c2} = 0$ , the free energy landscape is isotropic and for  $K_{c2} \neq 0$  local easy and hard axes emerge. Nevertheless, the second order cubic anisotropy has a negligible contribution to the magnon-magnon coupling as it does not further break the rotational symmetry of the free energy density.

Also,  $K_{c2}$  is not the (dominant) cause for the re-orientation of the magnetization for small external magnetic fields applied along the a.s.b. direction. Rather, this re-orientation can be understood based on Fig. 3(c) in the main text. In the a.s.b. configuration and for sufficiently small external magnetic fields, the antiparallel sublattice magnetizations can rigidly rotate towards the adjacent easy [111]-equivalent directions. This re-orientation is the cause of the minimum in  $f$  vs.  $H_0$  in Fig. 2(e) in the main text. In the e.a.s. configuration a rigid (uncanted) rotation of both antiparallel sublattice magnetizations towards the adjacent [111] directions is not possible and consequently we do not observe such re-orientation phenomena in Fig. 2(d) in the main text. Thus, the e.a.s. and a.s.b. directions are local magnetically easy and hard directions even for  $K_{c2} = 0$  where they are energetically degenerate (see Fig. S3(e)).

The parameters for our numerical calculations are given in Tab. S1. We treat the cubic anisotropies as free parameters, while the other parameters are either measured or taken from literature. We note that the similarity of  $K_{c1}$  and  $K_{c2}$  values and the decrease of  $K_{c1}$  and  $K_{c2}$  with increasing temperature are in agreement with expectations [12–14].

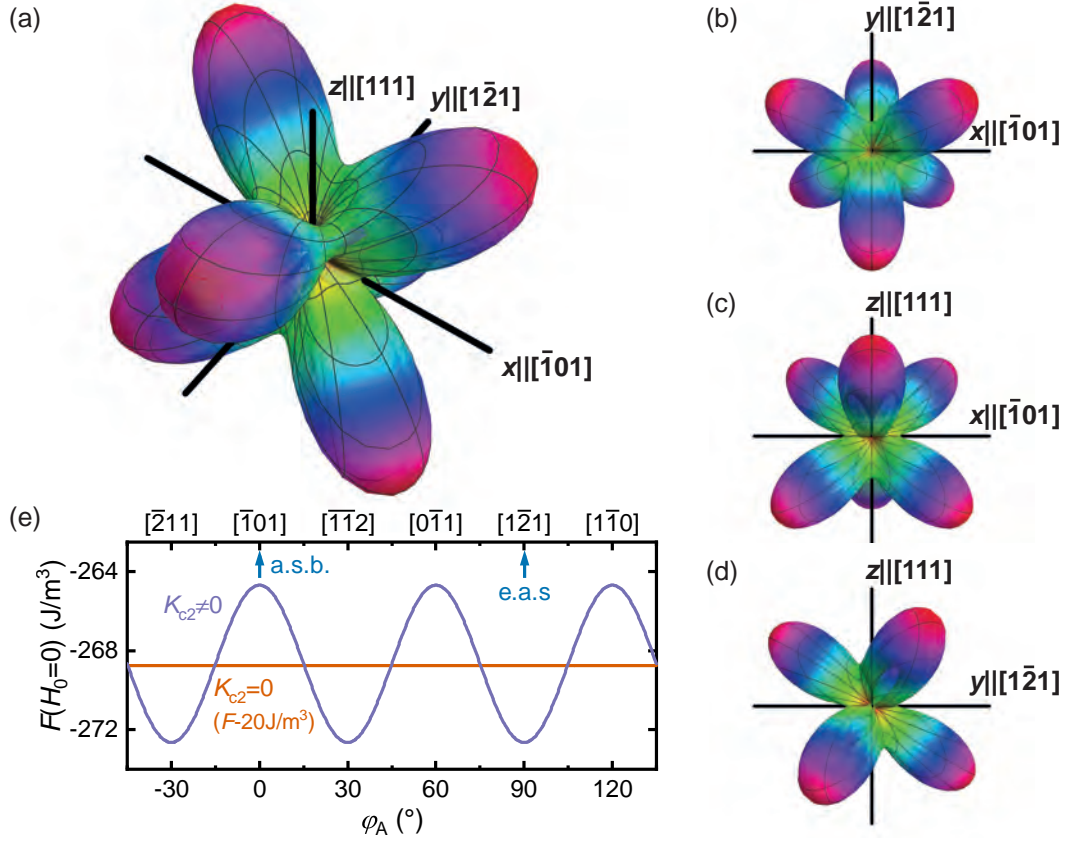

FIG. S3. (a) 3D illustration of the free energy density calculated with Eq. (S9). (b),(c),(d) Two-dimensional projections of the free energy density  $F$  as a function of the rotation angle  $\varphi_A$  in the  $xy$ -plane (disk plane,  $\theta_A = 90^\circ$ ). The angles  $\varphi_A$  and  $\theta_A$  denote the orientation of  $M_A$ , defined analogously to  $\varphi$  and  $\theta$  in Fig. 2(a) in the main text. The crystallographic axes are denoted at the top. For  $K_{c2} = 0$  (orange line), the  $xy$ -plane is isotropic. The blue arrows denote the axial symmetry broken axis (a.s.b.) and effectively axially symmetric axis (e.a.s.) where the measurements in the main text were performed.

TABLE S1. Used parameter sets for the numerical solving of the Landau-Lifshitz equation at  $T = 280$  K,  $T = 282$  K and  $T = 294$  K. For parameters with adjusted reference value (adj.), adjustments were less than 10% for better agreement with experimental data.

| Variable                | Value                  | Unit             | Variable                | Value                  | Unit             | Source                  |
|-------------------------|------------------------|------------------|-------------------------|------------------------|------------------|-------------------------|
| $M_{A0}$ (282 K)        | $1.606 \times 10^5$    | A/m              | $M_{B0}$ (282 K)        | $1.568 \times 10^5$    | A/m              | from Fig. S1, adj.      |
| $M_{A0}$ (280 K)        | $1.614 \times 10^5$    | A/m              | $M_{B0}$ (280 K)        | $1.568 \times 10^5$    | A/m              | from Fig. S1, adj.      |
| $M_{A0}$ (294 K)        | $1.500 \times 10^5$    | A/m              | $M_{B0}$ (294 K)        | $1.534 \times 10^5$    | A/m              | from Fig. S1, adj.      |
| $ \gamma_A $            | $1.754 \times 10^{11}$ | 1/Ts             | $ \gamma_B $            | $1.773 \times 10^{11}$ | 1/Ts             | [11, 12]                |
| $K_{c1}$ (280 K, 282 K) | -430                   | J/m <sup>3</sup> | $K_{c2}$ (280 K, 282 K) | -400                   | J/m <sup>3</sup> | adj.                    |
| $K_{c1}$ (294 K)        | -300                   | J/m <sup>3</sup> | $K_{c2}$ (294 K)        | -300                   | J/m <sup>3</sup> | adj.                    |
| $J$                     | $1.40 \times 10^{-4}$  | V s/(A m)        |                         |                        |                  | [11], adj.              |
| $\chi_a$ (282 K)        | 0.0077                 |                  |                         |                        |                  | from magnetometry, adj. |
| $\chi_a$ (280 K)        | 0.0079                 |                  |                         |                        |                  | from magnetometry, adj. |
| $\chi_a$ (294 K)        | -0.0080                |                  |                         |                        |                  | from magnetometry, adj. |

### CALCULATED ELLIPTICITIES

We numerically obtain the susceptibility  $\tilde{\chi}$  as explained above. We plot the ellipticity of the magnetization precession  $\epsilon = 1 - |\tilde{\chi}_{21}/\tilde{\chi}_{11}|$  in Fig. S4. An ellipticity of  $\epsilon = 0$  corresponds to circular precession and  $\epsilon = 1$  is equivalent to a linearly polarized magnon. Figure S4 shows that magnons are linearly polarized at the anti-crossing point, consistent with the small, but non-zero splitting observed along the e.a.s. direction. In Fig. S4(b) a more complicated evolution

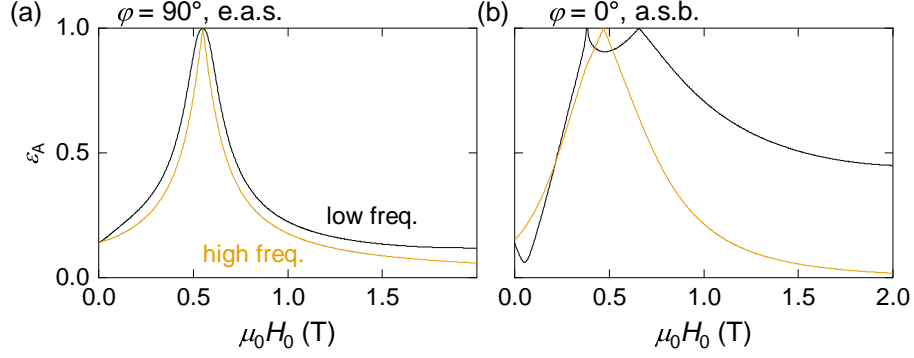

FIG. S4. Calculated ellipticities of the Gd-sublattice magnetization precession for the (a) effectively axial symmetric (e.a.s.) and the (b) axial symmetry broken (a.s.b.) cases at  $T = 282$  K. An ellipticity of  $\epsilon = 0$  corresponds to circular precession and  $\epsilon = 1$  corresponds to linear polarization.

of the ellipticity close to the hybridization point is observed. This complexity is rooted in several factors including evolution of the equilibrium configuration, ultrastrong nature of the hybridization, and a finite static susceptibility of the Gd sublattice.

#### DYNAMICS MATRICES AND PARAMETERS FOR THE ANALYTICAL MODEL

Here, we detail our analytic model and derivation of the coupled eigenmode frequencies. The re-orientation of the equilibrium magnetization direction with external magnetic applied along the a.s.b. direction is captured well by considering the e.a.s. and a.s.b. directions to bear uniaxial easy and hard anisotropies, respectively. In addition, for the a.s.b. configuration, we assume weak uniaxial anisotropies that break the axial symmetry about the applied field direction and thus underlie mode-coupling. Our carefully chosen model admits analytic solution, captures essential physics, and provides a general understanding of the key phenomena, which rely on broken symmetries and are not sensitive to the exact forms of the anisotropy.

The free energy density within our model thus reads as

$$F_m = -\mu_0 H_0 (M_{Az} + M_{Bz}) \mp K_A M_{Az}^2 \mp K_B M_{Bz}^2 + J \mathbf{M}_A \cdot \mathbf{M}_B + K_{ax} (M_{Ax}^2 + M_{Bx}^2) + K_{ay} (M_{Ay}^2 + M_{By}^2) + \frac{\mu_0}{2} (M_{Ax} + M_{Bx})^2, \quad (\text{S12})$$

where  $J$  ( $> 0$ ) parametrizes the inter-sublattice antiferromagnetic exchange,  $K_{A,B}$  ( $> 0$ ) account for easy-axis (upper sign) and hard-axis anisotropies (lower sign) along the applied field  $H_0 \hat{z}$ ,  $K_{ax,ay}$  anisotropy contributions allow for the axial symmetry-breaking about the  $z$ -axis when  $K_{ax} \neq K_{ay}$ , and the last term stems from shape anisotropy of our disk shaped sample corresponding to the demagnetization tensor elements  $N_x = 1$ ,  $N_{y,z} = 0$ . We further assume the following hierarchy of interactions  $J \gg K_{A,B} \gg |K_{ax,ay}|$ .

The equilibrium configuration is determined by minimizing the free energy density with respect to the sublattice magnetization directions, assumed spatially uniform within the macrospin approximation employed in our analysis. Due to the assumed hierarchy of interactions, the axial symmetry-breaking  $K_{ax,ay}$ -terms do not significantly affect the equilibrium state. The dynamical equations resulting from the Landau-Lifshitz equation

$$\frac{\partial \mathbf{M}_{A,B}}{\partial t} = -|\gamma_{A,B}| \left[ \mathbf{M}_{A,B} \times \left( -\frac{\partial F_m}{\partial \mathbf{M}_{A,B}} \right) \right] \quad (\text{S13})$$

are linearized about the equilibrium configuration, that defines a new primed coordinate system with the static magnetizations (nearly) collinear with  $\hat{z}'$ . As discussed below, except for a small range of applied fields in the hard-axis case, the static magnetizations are collinear with the  $z$ -axis and the two coordinate systems are identical. Switching to Fourier space via  $M_{Ax'} = m_{Ax'} e^{i\omega t}$  etc. and circular basis via  $m_{A\pm} = m_{Ax'} \pm i m_{Ay'}$ , we formulate the eigenvalue problem in terms of  $4 \times 4$  matrices:

$$\left( \tilde{P}_0 + \tilde{P}_a + \tilde{P}_d \right) \tilde{m} = 0, \quad (\text{S14})$$

where an overhead tilde identifies a 4-dimensional matrix or vector, and  $\tilde{m}^\top \equiv [m_{A+} \ m_{B+} \ m_{A-} \ m_{B-}]$ .

As we detail below,  $\tilde{P}_0$  is block-diagonal in  $2 \times 2$  sub-matrices and represents the two uncoupled eigenmodes delocalized over the two sublattices.  $\tilde{P}_a$  captures the off-diagonal, anisotropy-mediated contributions that cause an exchange-enhanced coupling between the two modes. Finally,  $\tilde{P}_d$  represents the shape anisotropy or dipolar interaction terms which are not exchange-enhanced, and thus do not significantly contribute to the observed coupling. This is because the  $2 \times 2$  sub-matrices that constitute  $\tilde{P}_d$  have a vanishing determinant. The corresponding physical interpretation is that close to compensation, i.e. when  $M_{A0} \approx M_{B0}$ , the static net magnetization nearly vanishes and only the small magnetic moment resulting from the dynamics causes dipolar interaction or shape anisotropy.

*Easy axis case.* – The static configuration for the range of experimentally relevant parameters and fields is given by  $\mathbf{M}_A = M_{A0}\hat{z}$  and  $\mathbf{M}_B = -M_{B0}\hat{z}$ , with the assumption  $M_{A0} > M_{B0}$ . The  $4 \times 4$  matrices that describe the dynamics and eigenmodes are given by:

$$\tilde{P}_0 = \begin{bmatrix} (-\omega + \Omega_A) & \Omega_{E1} & 0 & 0 \\ \Omega_{E2} & (\omega + \Omega_B) & 0 & 0 \\ 0 & 0 & (\omega + \Omega_A) & \Omega_{E1} \\ 0 & 0 & \Omega_{E2} & (-\omega + \Omega_B) \end{bmatrix}, \quad (S15)$$

$$\tilde{P}_a = \begin{bmatrix} \omega_{uA} & 0 & \omega_{cA} & 0 \\ 0 & \omega_{uB} & 0 & \omega_{cB} \\ \omega_{cA} & 0 & \omega_{uA} & 0 \\ 0 & \omega_{cB} & 0 & \omega_{uB} \end{bmatrix}, \quad (S16)$$

$$\tilde{P}_d = \frac{1}{2} \begin{bmatrix} \omega_{sA} & \omega_{sA} & \omega_{sA} & \omega_{sA} \\ \omega_{sB} & \omega_{sB} & \omega_{sB} & \omega_{sB} \\ \omega_{sA} & \omega_{sA} & \omega_{sA} & \omega_{sA} \\ \omega_{sB} & \omega_{sB} & \omega_{sB} & \omega_{sB} \end{bmatrix}. \quad (S17)$$

Here, we have defined  $\bar{K}_a \equiv (K_{ax} + K_{ay})/2$ ,  $\Delta\bar{K}_a \equiv (K_{ax} - K_{ay})/2$ ,  $\Omega_A \equiv |\gamma_A|(JM_{B0} + 2K_A M_{A0} + \mu_0 H_0)$ ,  $\Omega_B \equiv |\gamma_B|(JM_{A0} + 2K_B M_{B0} - \mu_0 H_0)$ ,  $\Omega_{E1} \equiv |\gamma_A|JM_{A0}$ ,  $\Omega_{E2} \equiv |\gamma_B|JM_{B0}$ ,  $\omega_{uA,uB} \equiv 2|\gamma_{A,B}|\bar{K}_a M_{A0,B0}$ ,  $\omega_{cA,cB} \equiv 2|\gamma_{A,B}|\Delta\bar{K}_a M_{A0,B0}$ , and  $\omega_{sA,sB} \equiv |\gamma_{A,B}|\mu_0 M_{A0,B0}$ . Note that in our analysis, we account for the dependence of Gd-sublattice saturation magnetization, represented here by  $M_{A0}$ , on the applied field via a small but finite static susceptibility  $\chi_a$  (see Table S2).

*Hard axis case.* – For the experimentally relevant parameters and within the assumed hierarchy of interactions in the present analysis, the equilibrium configuration is given by:

$$\vartheta = \cos^{-1} \left( \frac{2\mu_0 H_0 \Delta\bar{M}_0}{4\bar{L} - \chi_a \mu_0 H_0^2} \right), \quad \text{for } \frac{2\mu_0 H_0 \Delta\bar{M}_0}{4\bar{L} - \chi_a \mu_0 H_0^2} < 1, \quad (S18)$$

$$= 0 \quad \text{for } \frac{2\mu_0 H_0 \Delta\bar{M}_0}{4\bar{L} - \chi_a \mu_0 H_0^2} \geq 1, \quad (S19)$$

$$\phi = \frac{\mu_0 H_0 \bar{M}_0 \sin \vartheta - \Delta\bar{L} \sin 2\vartheta}{2JM_{A0}M_{B0}} \ll 1, \quad \text{for } \frac{2\mu_0 H_0 \Delta\bar{M}_0}{4\bar{L} - \chi_a \mu_0 H_0^2} < 1, \quad (S20)$$

$$= 0, \quad \text{for } \frac{2\mu_0 H_0 \Delta\bar{M}_0}{4\bar{L} - \chi_a \mu_0 H_0^2} \geq 1, \quad (S21)$$

where we define  $\bar{M}_0 \equiv (M_{A0} + M_{B0})/2$ ,  $\Delta\bar{M}_0 \equiv (M_{A0} - M_{B0})/2$ ,  $\bar{L} \equiv (K_A M_{A0}^2 + K_B M_{B0}^2)/2$ , and  $\Delta\bar{L} \equiv (K_A M_{A0}^2 - K_B M_{B0}^2)/2$ . Here,  $\vartheta - \phi \approx \vartheta$  is the angle that static A-sublattice magnetization makes with the applied field, and  $2\phi \approx 0$  is the angle between the two static sublattice magnetizations. Once again we have accounted for the small but finite static susceptibility  $\chi_a$  of the Gd-sublattice. Thus we see that at low fields, the two nearly anticollinear sublattices make an angle with the applied magnetic field. With increasing field, the sublattices rotate to align with it until they become perfectly collinear with the applied field.

The matrices describing the dynamics have a structure similar to Eqs. (S15) - (S17). We first consider the low-field regime when sublattice magnetizations are not aligned with the applied field.  $\tilde{P}_d$  is still given by Eq. (S17), while  $\tilde{P}_0$  is given by Eq. (S15) with the replacements:  $\Omega_A \equiv |\gamma_A|(JM_{B0} - 2K_A M_{A0} \cos 2\vartheta + \mu_0 H_0 \cos \vartheta)$  and  $\Omega_B \equiv |\gamma_B|(JM_{A0} - 2K_B M_{B0} \cos 2\vartheta - \mu_0 H_0 \cos \vartheta)$ . In this configuration, the  $K_{A,B}$  anisotropy contributions, that are axially symmetric about the applied field direction, break axial symmetry about the static magnetizations resulting in mode

coupling. Therefore, these dominate the mode-coupling and consequently,  $\tilde{P}_a$  reads:

$$\tilde{P}_a = - \begin{bmatrix} \omega_{hA} & 0 & \omega_{hA} & 0 \\ 0 & \omega_{hB} & 0 & \omega_{hB} \\ \omega_{hA} & 0 & \omega_{hA} & 0 \\ 0 & \omega_{hB} & 0 & \omega_{hB} \end{bmatrix}, \quad (S22)$$

where  $\omega_{hA,hB} \equiv \sin^2 \vartheta |\gamma_{A,B}| K_{A,B} M_{A0,B0}$ .

In the high-field regime, where the anticrossing occurs,  $\tilde{P}_0$  is again given by Eq. (S15) with the replacements:  $\Omega_A \equiv |\gamma_A|(JM_{B0} - 2K_A M_{A0} + \mu_0 H_0)$  and  $\Omega_B \equiv |\gamma_B|(JM_{A0} - 2K_B M_{B0} - \mu_0 H_0)$ .  $\tilde{P}_a$  and  $\tilde{P}_d$  retain their forms given by Eqs. (S16) and (S17), respectively. Thus, we see that the weak  $K_{ax,ay}$  contributions underlie the observed anticrossing and hybridization since it occurs in the regime when the static sublattice magnetizations are perfectly collinear with the applied field.

TABLE S2. Parameters used in the analytical calculations for  $T = 282$  K. For parameters with adjusted reference value (adj.), adjustments were less than 10% for better agreement with experimental data.

| Variable     | Value                  | Unit      | Variable     | Value                  | Unit      | Source             |
|--------------|------------------------|-----------|--------------|------------------------|-----------|--------------------|
| $M_{A0}$     | $1.602 \times 10^5$    | A/m       | $M_{B0}$     | $1.576 \times 10^5$    | A/m       | from Fig. S1, adj. |
| $ \gamma_A $ | $1.754 \times 10^{11}$ | 1/Ts      | $ \gamma_B $ | $1.773 \times 10^{11}$ | 1/Ts      | [11, 12]           |
| $K_A$        | $7.2 \times 10^{-9}$   | V s/(A m) | $K_B$        | $2 \times 10^{-8}$     | V s/(A m) | [11], adj.         |
| $K_a$        | $3.58 \times 10^{-8}$  | V s/(A m) |              |                        |           | adj.               |
| $J$          | $1.44 \times 10^{-4}$  | V s/(A m) |              |                        |           | [11], adj.         |
| $\chi_a$     | 0.0078                 |           |              |                        |           | magnetometry, adj. |

For the analytical calculations, we employ the parameters given in Table S2. All parameters are either measured or taken from literature. The minor difference between the parameters used for the analytical and the numerical calculations stems from the different forms of the free energy densities. Table S2 shows that the anisotropy parameters employed to reproduce the experimental curves do not respect the hierarchy of interactions assumed, in order to enable an analytic solution, herein. This underlies the relatively minor deviations of the eigenmode frequencies evaluated within our analytic model from their experimentally measured counterparts.

## ANALYTIC EXPRESSION FOR EXCHANGE-ENHANCED FREQUENCY SPLITTING

We now derive an analytic expression for the frequency splitting due to mode-coupling at the field value where the uncoupled modes would become degenerate. To this end, we solve the eigenvalue problem defined by:

$$(\tilde{P}_0 + \tilde{P}_a) \tilde{m} = 0, \quad (S23)$$

where  $\tilde{P}_0$  and  $\tilde{P}_a$  are given by Eqs. (S15) and (S16), respectively. As described in the previous section, this matrix structure captures both easy-axis and hard-axis configurations with slightly different definitions for  $\Omega_{A,B}$ . This assumes the sublattice magnetizations to be collinear with the applied field direction, which is the case in our experiment, as evident from the data and our detailed theoretical models. Furthermore, we have disregarded the contribution ( $\tilde{P}_d$ ) of shape anisotropy or dipolar interaction since it is not exchange-enhanced and is thus negligible. This assumption is also validated by numerical evaluation of frequency splitting employing the fully detailed model.

The secular equation for the eigenvalue problem posed in Eq. (S23) is quadratic in  $\omega^2$ :

$$\omega^4 - b\omega^2 + c = 0, \quad (S24)$$

where

$$b \equiv \Omega_1^2 + \Omega_2^2 - \omega_{cA}^2 - \omega_{cB}^2 - 2\Omega_{E1}\Omega_{E2}, \quad (S25)$$

$$c \equiv \Omega_1^2\Omega_2^2 - \Omega_1^2\omega_{cB}^2 - \Omega_2^2\omega_{cA}^2 + \omega_{cA}^2\omega_{cB}^2 + \Omega_{E1}^2\Omega_{E2}^2 - 2\Omega_{E1}\Omega_{E2}\omega_{cA}\omega_{cB} - 2\Omega_{E1}\Omega_{E2}\Omega_1\Omega_2. \quad (S26)$$

Here, we have defined  $\Omega_{1,2} \equiv \Omega_{A,B} + \omega_{uA,uB}$  for convenience. We are interested in the two positive solutions  $\omega_{1,2}$ , with  $\omega_1 \geq \omega_2$ , of the above secular equation. Employing the expression for roots of a quadratic equation, we have:

$$\omega_1^2 - \omega_2^2 = \sqrt{b^2 - 4c}. \quad (S27)$$

Now we employ the condition that in the absence of coupling, i.e. when  $\omega_{cA,cB} = 0$ , the modes are degenerate, i.e.  $\omega_1 = \omega_2$ . The above equation thus simplifies to:

$$\omega_1^2 - \omega_2^2 = \left[ 4\Omega_{E1}\Omega_{E2}(\omega_{cA} + \omega_{cB})^2 - 2(\Omega_1^2 - \Omega_2^2)(\omega_{cA}^2 - \omega_{cB}^2) \right]^{\frac{1}{2}}, \quad (S28)$$

$$\Rightarrow \omega_1 - \omega_2 = \frac{\left[ 4\Omega_{E1}\Omega_{E2}(\omega_{cA} + \omega_{cB})^2 - 2(\Omega_1^2 - \Omega_2^2)(\omega_{cA}^2 - \omega_{cB}^2) \right]^{\frac{1}{2}}}{\omega_1 + \omega_2}, \quad (S29)$$

retaining terms to the lowest order in  $\omega_{cA,cB}$ . It is sufficient to evaluate  $\omega_1 + \omega_2$  disregarding mode-coupling, i.e. assuming  $\omega_{cA,cB} = 0$ , for obtaining the coupling-mediated frequency splitting to the lowest order in  $\omega_{cA,cB}$ .

In order to obtain  $\omega_1 + \omega_2$ , we employ the properties of our quadratic secular equation (S24) roots  $\omega_1^2 + \omega_2^2 = b$  and  $\omega_1^2\omega_2^2 = c$  to obtain:

$$\omega_1 + \omega_2 = \sqrt{\omega_1^2 + \omega_2^2 + 2\omega_1\omega_2}, \quad (S30)$$

$$= \sqrt{b + 2\sqrt{c}}, \quad (S31)$$

$$= \sqrt{\Omega_1^2 + \Omega_2^2 - 2\Omega_{E1}\Omega_{E2} + 2|\Omega_1\Omega_2 - \Omega_{E1}\Omega_{E2}|}, \quad (S32)$$

where we have employed Eqs. (S25) and (S26) in conjunction with the condition of vanishing coupling in making the last simplification. Invoking the hierarchy of interactions, we replace  $\Omega_{1,2}$  with  $\Omega_{A,B}$  in the ongoing analysis. Employing Eq. (S19), it can be shown that  $\Omega_A\Omega_B \geq \Omega_{E1}\Omega_{E2}$  for the equilibrium magnetizations to be collinear with the applied field, as has been assumed herein. Thus, from Eqs. (S29) and (S32), we obtain:

$$\omega_1 - \omega_2 = 2\pi\Delta f_{\text{res}} = \left[ \frac{4\Omega_{E1}\Omega_{E2}(\omega_{cA} + \omega_{cB})^2 - 2(\Omega_A^2 - \Omega_B^2)(\omega_{cA}^2 - \omega_{cB}^2)}{(\Omega_A + \Omega_B)^2 - 4\Omega_{E1}\Omega_{E2}} \right]^{\frac{1}{2}}, \quad (S33)$$

which is our generic result for the desired frequency splitting  $\Delta f_{\text{res}}$ .

We now employ the general expression obtained above to achieve specific results for the two cases of interest. Accounting for the hierarchy of interactions, the frequency splitting expression reduces to:

$$2\pi\Delta f_{\text{res}} = \left[ \frac{8J(\Delta\bar{K}_a)^2 \left\{ (|\gamma_A|M_{A0} + |\gamma_B|M_{B0})^2 2|\gamma_A||\gamma_B|M_{A0}M_{B0} - (|\gamma_A|^2M_{A0}^2 - |\gamma_B|^2M_{B0}^2)(|\gamma_A|^2M_{B0}^2 - |\gamma_B|^2M_{A0}^2) \right\}}{J(|\gamma_A|M_{B0} - |\gamma_B|M_{A0})^2 + 2\{|\gamma_A|M_{B0} + |\gamma_B|M_{A0}\}\{\mu_0H_0(|\gamma_A| - |\gamma_B|) \pm 2(|\gamma_A|K_A M_{A0} + |\gamma_B|K_B M_{B0})\}} \right]^{\frac{1}{2}}, \quad (S34)$$

where upper and lower signs correspond to easy- and hard-axis configurations, respectively. Assuming  $\gamma_A = \gamma_B = \gamma$ ,  $K_A = K_B = K$ ,  $K_{ax} = K_a$ , and  $K_{ay} = 0$  such that  $\Delta\bar{K}_a = K_a/2$ , we obtain:

$$2\pi\Delta f_{\text{res}} = \left[ \frac{2J|\gamma|^2K_a^2 \left\{ (M_{A0} + M_{B0})^2 2M_{A0}M_{B0} + (M_{A0}^2 - M_{B0}^2)^2 \right\}}{J(M_{A0} - M_{B0})^2 \pm 4K(M_{A0} + M_{B0})^2} \right]^{\frac{1}{2}}. \quad (S35)$$

Furthermore, we may assume  $M_{A0} - M_{B0} \ll M_{A0}, M_{B0}$  close to the compensation temperature such that  $M_{A0} \approx M_{B0} \equiv M_0$ :

$$2\pi\Delta f_{\text{res}} = |\gamma||K_a|M_0 \sqrt{\frac{16JM_0^2}{J(M_{A0} - M_{B0})^2 \pm 16KM_0^2}}. \quad (S36)$$

The expression thus obtained clearly demonstrates the exchange-enhancement effect for the easy-axis configuration (upper sign). The bare coupling rate  $\omega_c = |\gamma||K_a|M_0$  is thus enhanced by the factor under square root. A maximum enhancement of  $\sqrt{J/K}$  is achieved when the two sublattices are exactly compensated, i.e. when  $M_{A0} = M_{B0}$ .

However, Eq. (S36) results in an imaginary enhancement factor for the hard-axis configuration (lower sign) too close to the compensation point. This apparent anomaly arises because our assumption of equilibrium magnetizations being collinear with the applied field requires a small but finite  $M_{A0} - M_{B0}$  [see Eq. (S19)]. Thus, the ferrimagnet is not allowed to be perfectly compensated within our assumptions. There can be no anticrossing between the two

modes in the hard-axis configuration with a collinear ground state for a perfectly compensated ferrimagnet, or an antiferromagnet for that matter. In order to emphasize that there is no anomaly and obtain a form similar to the easy-axis case, the frequency splitting in the hard-axis case may be expressed as:

$$2\pi\Delta f_{\text{res}} = \omega_c \sqrt{\frac{16JM_0^2}{J(M_{A0} - M_{B0})^2 + F_{\text{eq}}}}, \quad (\text{S37})$$

where  $F_{\text{eq}} = -16KM_0^2$  is an equivalent free energy density. Furthermore, the sublattice magnetizations imbalance is such that  $J(M_{A0} - M_{B0})^2 + F_{\text{eq}}$  is positive and comparable to  $|F_{\text{eq}}|$ .

## QUALITATIVE DISCUSSION OF ESSENTIAL PHYSICS

In the previous two sections, we have employed a simplified and analytically tractable model for the ferrimagnet to understand its dynamical eigenmodes and their frequency splitting at the anticrossing point. To this end, we employed the classical Landau-Lifshitz (LL) framework obtaining results in good agreement with our experimental data (Figs. 2(d) and (e) in main text). Capitalizing on these mathematically rigorous results obtained above, we now discuss the essential physics qualitatively highlighting the key ingredients and phenomena one by one. The quantum picture representing the eigenmodes as magnons [15], discussed already in the main text (Fig. 1 in main text), is particularly convenient for developing an intuition regarding the key phenomena discussed herein. Therefore, we will here switch back and forth between the classical and quantum pictures as per convenience. Of course, the two descriptions are equivalent for the case at hand. Furthermore, for the sake of completeness, we repeat part of the discussion that is already presented in the main text.

*Mode coupling, violation of spin conservation, and axial anisotropy.* The two eigenexcitations of the ferrimagnetic collinear ground states considered herein are the spin-up and -down magnons in the quantum picture (Fig. 1 in main text). These magnons possess unit ( $\hbar$ ) net spins in opposite directions collinear with the equilibrium sublattice magnetizations. We refer to this direction as the magnon spin axis. When two modes couple, it means that energy can be transferred from one to the other. In the quantum parlance, this implies that one mode can be converted into the other. This mode interconversion, and thus the coupling, needs to respect the conservation laws in the system. As a result, a spin-up magnon is not allowed to couple with (transmute into) its spin-down counterpart, if the spin along the magnon spin axis is a conserved quantity. This is why the magnon-magnon coupling that we observe necessarily stems from spin-nonconserving mechanisms [15] and cannot be anticipated from the isotropic exchange interaction. Since the conservation of spin along a direction is mathematically a consequence of axial symmetry about this direction, the spin-nonconserving mechanism required for the magnon-magnon coupling is provided by an anisotropy about the magnon spin axis. As shown by our analysis above, the axial anisotropy manifests itself in the LL theory as nonzero off-diagonal elements captured by Eq. (S16) that couple the two modes.

*Anisotropy symmetry.* We note that the exact form of the anisotropy is not important as long as it breaks the axial symmetry. The latter property ensures nonzero elements in the off-diagonal coupling matrix. For any anisotropy landscape, the dynamical matrices describing the eigenmodes will assume a structure similar to the ones presented above. This is why our assumed simple uniaxial anisotropies (Eq. (S12)) are able to capture the dynamical effects of the realistic cubic magnetocrystalline anisotropy rather well.

*Antiferromagnetic magnons and exchange-enhancement.* The magnetocrystalline anisotropy in GdIG is very weak and cannot be expected to result in strong observable effects on its own, and hence is typically disregarded. This is indeed true for GdIG far away from compensation temperature. However, at and around the compensation point, the two sublattice magnetizations become nearly equal and the spatially uniform modes of the ferrimagnet behave like in an antiferromagnet (AFM) [15]. The special character of the AFM magnons, arising from the well-known strong quantum fluctuations [16], leads to a drastic enhancement of the anisotropy-mediated mode-coupling as described in the following. On an average, the antiferromagnetic spin-up magnon is composed of a large up spin, say  $N$ , on one sublattice and another large, opposite down spin ( $N - 1$ ) on the other [16]. Thus, despite its unit net spin, it bears rather large ( $\sim \sqrt{J/K}$ ) spins on each of the sublattices. The same is true for the antiferromagnetic spin-down magnon with the roles of sublattices reversed. Any interaction which is mediated by the sublattice, instead of the net, spin is therefore amplified by the large sublattice spin ( $\sim \sqrt{J/K}$ ) [16]. This effect is termed exchange-enhancement since it is mediated by and increases with the antiferromagnetic exchange interaction. It is evident from Eq.(S12) that the anisotropy-mediated mode-coupling is governed by the sublattice magnetizations or spins (free energy  $\sim M_{Ax}^2 + M_{Bx}^2$ ) and not the net magnetization or spin ( $\sim (M_{Ax} + M_{Bx})$ ). Thus, the mode-coupling is accordingly amplified via the

exchange-enhancement effect (Eq. (S37)) when the ferrimagnet is close to its compensation temperature and behaves like an AFM.

*Demagnetization fields.* The discussion above also clarifies why the dipolar interaction or demagnetization fields do not play an important role in our experimental observations. This contribution does provide a small but nonzero mode coupling and has been accounted for in our analysis (Eq. (S12)). However, this interaction is mediated by the net magnon spin (free energy  $\sim (M_{Ax} + M_{Bx})^2$ ) and is thus not exchange-enhanced. Furthermore, it is weak to begin with since the total magnetization around the compensation point is small. This is also encoded mathematically in the dynamical matrix structure (Eq. (S17)) resulting from the dipolar interaction as discussed earlier. As a result, the mode-coupling caused by the dipolar fields is negligibly small for the case at hand.

---

\* Lukas.Liensberger@wmi.badw.de

† Akashdeep.Kamra@ntnu.no

‡ Mathias.Weiler@wmi.badw.de

- [1] G. F. Dionne, *Magnetic Oxides* (Springer US, Boston, MA, 2009).
- [2] S. Koohpayeh, Single crystal growth by the traveling solvent technique: A review, *Progress in Crystal Growth and Characterization of Materials* **62**, 22 (2016).
- [3] G. F. Dionne, Molecular Field Coefficients of Substituted Yttrium Iron Garnets, *Journal of Applied Physics* **41**, 4874 (1970).
- [4] G. F. Dionne, Molecular Field and Exchange Constants of  $Gd^{3+}$ -Substituted Ferrimagnetic Garnets, *Journal of Applied Physics* **42**, 2142 (1971).
- [5] E. C. Stoner and E. P. Wohlfarth, A Mechanism of Magnetic Hysteresis in Heterogeneous Alloys, *Philosophical Transactions of the Royal Society A: Mathematical, Physical and Engineering Sciences* **240**, 599 (1948).
- [6] H. Maier-Flaig, S. T. B. Goennenwein, R. Ohshima, M. Shiraishi, R. Gross, H. Huebl, and M. Weiler, Note: Derivative divide, a method for the analysis of broadband ferromagnetic resonance in the frequency domain, *Review of Scientific Instruments* **89**, 076101 (2018).
- [7] S. Klingler, V. Amin, S. Geprägs, K. Ganzhorn, H. Maier-Flaig, M. Althammer, H. Huebl, R. Gross, R. D. McMichael, M. D. Stiles, S. T. Goennenwein, and M. Weiler, Spin-Torque Excitation of Perpendicular Standing Spin Waves in Coupled YIG/Co Heterostructures, *Physical Review Letters* **120**, 127201 (2018).
- [8] D. Polder, VIII. On the theory of ferromagnetic resonance, *The London, Edinburgh, and Dublin Philosophical Magazine and Journal of Science* **40**, 99 (1949).
- [9] L. Dreher, M. Weiler, M. Pernpeintner, H. Huebl, R. Gross, M. S. Brandt, and S. T. B. Goennenwein, Surface acoustic wave driven ferromagnetic resonance in nickel thin films: Theory and experiment, *Physical Review B* **86**, 134415 (2012).
- [10] J. A. Osborn, Demagnetizing Factors of the General Ellipsoid, *Physical Review* **67**, 351 (1945).
- [11] S. Geschwind and L. R. Walker, Exchange Resonances in Gadolinium Iron Garnet near the Magnetic Compensation Temperature, *Journal of Applied Physics* **30**, S163 (1959).
- [12] G. P. Rodrigue, H. Meyer, and R. V. Jones, Resonance Measurements in Magnetic Garnets, *Journal of Applied Physics* **31**, S376 (1960).
- [13] B. A. Calhoun and M. J. Freiser, Anisotropy of Gadolinium Iron Garnet, *Journal of Applied Physics* **34**, 1140 (1963).
- [14] P. Hansen, Ferromagnetic Resonance in Ruthenium-Doped Gadolinium Iron Garnet, *Physical Review B* **5**, 3737 (1972).
- [15] A. Kamra, U. Agrawal, and W. Belzig, Noninteger-spin magnonic excitations in untextured magnets, *Physical Review B* **96**, 020411(R) (2017).
- [16] A. Kamra, E. Thingstad, G. Rastelli, R. A. Duine, A. Brataas, W. Belzig, and A. Sudbø, Antiferromagnetic Magnons as Highly Squeezed Fock States underlying Quantum Correlations, *arXiv:1904.04553*, 1 (2019).
